# Supplementary material for: On the convergence of dynamic implementations of Hamiltonian Monte Carlo and No U-Turn Samplers
Source: arXiv:2307.03460 source file (2024-10-18)
Supplement: Supplementary file 1 [file energy_check.tex]

In Section 3 %[[\ref{sec:nuts-its-invariance}]]
we defined the exact NUTS variant under study in this paper without the energy checks that are a feature of almost all practical implementations of NUTS.
Here we briefly describe these checks and present our rationale for omitting them.

Recall the formulation (12) %[[\eqref:eq:scrU]]
for the U-turn checks in terms of the sets %[[\ref{sec:nuts-its-invariance]]
\begin{gather}
    \scrU_{k,l,+}^{(K)} = \{ v\in B_{K}:\ee p_{i_{+}(K,k,l,v)}^\top (q_{i_{+}(K,k,l,v)} - q_{i_{-}(K,k,l,v)}) < 0 \} \eqsp,
    \\
    \scrU_{k,l,-}^{(K)} = \{v\in B_{K}: \ee p_{i_{-}(K,k,l,v)}^\top (q_{i_{+}(K,k,l,v)} - q_{i_{-}(K,k,l,v)}) < 0 \} \eqsp,
\end{gather}
where
$$i_{-}(K,k,l,v)=-T_-^{(K)}(v)+(l-1) 2^k,\qquad i_{+}(K,k,l,v)=-T_-^{(K)}(v) + l 2^k-1 $$
for $v\in B_{K}$, $K\in [\Kmax]$, $k\in [K-1]$ and $l\in [2^{K-k}]$, in Section 3.
These sets define the termination criterion for the trajectory construction via (13). %[[\eqref{eq:nuts-stopping}]]
In Stan, the \emph{energy checks} augment the termination criterion by adding additional checks of the form
\begin{equation}
    \label{eq:stan_energy_check}
    \mathscr{E}_k^{(K)} = \{ v \in B_K: \ee H(q_j, p_j) < H(q_0, p_0) - \Delta_{\mathrm{max}} \textit{ for some } j \in B_K(v) \},
\end{equation}
where $\Delta_{\mathrm{max}} > 0$ is a fixed large constant.
In Stan, $\Delta_{\mathrm{max}}$ has the hard-coded value $\Delta_{\mathrm{max}} = 1000$.
These checks ensure that trajectory construction is terminated in the case that the leapfrog integrator becomes unstable and fails to conserve energy even approximately on the current trajectory.
We remark that the primary purpose of these checks is diagnostic -- if energy conservation fails by a margin of $1000$, it is very likely that an U-turn also occurs on the same trajectory.
Thus the trajectories on which the energy check fails are called divergent.

The reason we have omitted the energy check from our theoretical analysis is that the check \eqref{eq:stan_energy_check} does not preserve the symmetry of the trajectory construction in the sense of Corollary 3 %[[\Cref{cor:trajectory-invariance-symmetric}
and the algorithm with the energy check \eqref{eq:stan_energy_check} is biased -- though with the value $\Delta_{\mathrm{max}} = 1000$ the bias is practically negligible\footnote{In our experiments we had to set $\Delta_{\mathrm{max}} \approx 1$ in order to see appreciable bias on a Gaussian target distribution.}.
Finally, we remark that as in \cite{sherlock2023apogee} it is simple to fix the energy check by replacing \eqref{eq:stan_energy_check} by
\begin{equation}
    \label{eq:fixed_energy_check}
    \tilde{\mathscr{E}}_k^{(K)} = \{ v \in B_K: \ee \big|H(q_j, p_j) - H(q_{j'}, p_{j'})| < - \Delta_{\mathrm{max}} \textit{ for some } j, j' \in B_K(v) \}.
\end{equation}
