# Supplementary material for: On the convergence of dynamic implementations of Hamiltonian Monte Carlo and No U-Turn Samplers
Source: arXiv:2307.03460 source file (2024-10-18)
Supplement: Supplementary file 2 [file equivalence_algorithm.tex]

  %il semble que le stoppping time ne fasse pas exactement ce qu'on veut, possibilité de sampler dans un set avec Uturn

  \begin{algorithm}
      \caption{
          Practical implementation for the no U-turn HMC proposal
      }
      \label{alg:practical}
      \begin{algorithmic}[1]
          \Statex \textbf{Input}
              initial position and momentum $\theta_0=(q_0, p_0) \in (\Rset^d)^2$,
              maximum tree height $\Kmax$,
              leapfrog parameters
          \State $\theta^-_0 \gets \theta_0$, $\theta^+_0 \gets \theta_0$,$\theta_0\gets \theta_0$, $k\gets0$, $s_0\gets 1$, $\Sigma(\pi)_0\gets \tpi(\theta_0)$
        
          \While {$s_k=1$ and $k < \Kmax$}
              \State $V_k \sim \operatorname{Ber}(\tfrac{1}{2})$,\ee $\theta_{k+1}\gets \theta_k$
              \If {$V_k=0$}
                \State $\theta^-_{k+1},\_,\theta'_k,\Sigma(\pi)'_k,s'_k\gets $ BuildTree($\theta^-,-1,k$)
              \Else
                \State $\_,\theta^+_{k+1},\theta'_k,\Sigma(\pi)_k',s'_k\gets $BuildTree($\theta^+,1,k$)
              \EndIf
              \If {$s'_k=1$}
                \State with probability $\min(1,\frac{\Sigma(\pi)'_k}{\Sigma(\pi)_k})$, set $ \theta_{k+1}\gets \theta'_k$
      \EndIf
      
    \State $\Sigma(\pi)_{k+1}\gets \Sigma(\pi)_k+\Sigma(\pi)_k'$
    \State $q^+_{k+1},p^+_{k+1} \gets \theta^+_{k+1}$, $q^-_{k+1},p^-_{k+1}\gets \theta^-_{k+1} $
    \State $s_{k+1}\gets s'_k  \mathbbm{1}[(q^+_{k+1} - q^-_{k+1}).p^-_{k+1}\geq 0]  \mathbbm{1}[(q^+_{k+1} -q^-_{k+1}).p^+_{k+1}\geq 0]$,
      \State $k\gets k+1$
          \EndWhile
      \State \textbf{return} $\theta_k'$
          \State \textbf{function} BuildTree($\theta,v,k$)
          \If {$k=0$}
    \State $\theta' \gets Leapfrog(\theta,vh)$
    \State $\Sigma(\pi)'\gets \tpi(\theta'), \ee s'\gets 1$
    \State \textbf{return} $\theta',\theta',\Sigma(\pi)',s'$
    
          \Else
            \State $\theta^-,\theta^+,\theta',\Sigma(\pi)',s'\gets$ BuildTree($\theta,v,k-1$)
           
          \If {$s'=1$}
          \If {$v=0$}
                \State $\theta^-,\_,\theta'',\Sigma(\pi)'',s''\gets $ Buildtree($\theta^-,v,k-1$)
              \Else
                \State $\_,\theta^+,\theta'',\Sigma(\pi)'',s''\gets $Buildtree($\theta^+,v_k,k$)
              \EndIf
              
             \State with probability $\frac{\Sigma(\pi)'}{\Sigma(\pi)'+\Sigma(\pi)''}$, set $ \theta'\gets \theta''$
             \State $\Sigma(\pi)'\gets \Sigma(\pi)'+\Sigma(\pi)''$, $k\gets k+1$
    \State $q^+,p^+ \gets \theta^+$, $q^-,p^-\gets \theta^- $
    \State $s'\gets s''  \mathbbm{1}[(q^+ - q^-).p^-\geq 0]  \mathbbm{1}[(q^+ -q^-).p^+\geq 0]$
    \EndIf
    \State \textbf{return} $\theta',\theta',\Sigma(\pi),s'$
    \EndIf

      \end{algorithmic}
  \end{algorithm}
   The goal of this section is to understand the structure behind the construction of the index selection kernel of the NUTS sampler $\rmq_h$. 
   As a corollary, we will see the link between \Cref{alg:practical} and its simplified version Algorithm 1 [[\ref{alg:nuts-doubling}]]. (à voir avec Alain si on insert ou pas des variables aléatoires)
  
   First, denoting by $\theta^-_k,\theta^+_k$ the variables at step $k$ in \Cref{alg:practical} for $k\in [1,\Kmax]$, 
   we remark that at line 5 and 7, we have $\theta^-_{k+1}=\Phiverlet[h][-2^k](\theta^-_k)$ and $\theta^+_{k+1}=\Phiverlet[h][2^k](\theta^+_k)$ respectively thank to the Buildtree recurcive structure when there is no U turn.
    Denoting by $I_k$ the set generated at step $k$ in Algorithm 1 [[\ref{alg:nuts-doubling}]], we have
      $$\theta^-_k=\Phiverlet[h][j^-_k](q_0,p_0),\ee\theta^+=\Phiverlet[h][j^+_k](q_0,p_0),\ee \min I_k=j^-_k,\ee \max I_k=j^+_k\ee .$$
     since line 5 and 7 are equivalent to add $2^k$ elements on the left or on the right to $I_k$ (the set related to the trajectory).
  \begin{lemma}
      The update of the proposition $q_{j_f} $ Line 18 in Algorithm 1 [[\ref{alg:nuts-doubling}]] and the update of the proposition $\theta_{k}$ line 10 in \Cref{alg:practical} are equivalent.
  \end{lemma}
  \begin{proof}
      In \Cref{alg:practical}, checking $s_k'=1$ (line 9) is equivalent to check $\operatorname{NoUTurns}(I^{\text{new}}_{k}, \{q_\ell, p_\ell : \ell \in I^{\text{new}}_{k} \})$ is False and $\mathbbm{1}[(q^\epsilon_{k+1} - q^\epsilon_{k}).p^\epsilon_{k}\geq 0]  \mathbbm{1}[(q^\epsilon_{k} -q^\epsilon_{k}).p^\epsilon_{k}\geq 0]$ with $\epsilon\in \{+,-\}$ according to the value of $V_k$.
      Checking $s_k=1$ (line 2) is equivalent to check $s_{k-1}'=1$ and $\mathbbm{1}[(q^+_{k+1} - q^-_{k+1}).p^-_{k+1}\geq 0]  \mathbbm{1}[(q^+_{k} -q^-_{k}).p^+_{k}\geq 0]$, if $s_{k-1}=1$.
      When we check the condition $s_k'=1$ we have already $s_k=1$, thus checking $ s_{k}'=1$ is equivalent to check if $\operatorname{NoUTurns}(I_{k+1}', \{q_\ell, p_\ell : \ell \in I_{k+1}'\})$ is False which is the condition line 17 in Algorithm 1 [[\ref{alg:nuts-doubling}]].
  \end{proof}
  
  \begin{definition}
  A triplet $(D,F_{\text{old}},F_{\text{new}})$ is Binary Russian Doll (BRD),
  if $D\subset \mathcal{P}(\mathbb{Z}),\ee F_{\text{old}},F_{\text{new}} \in (\mathcal{P}(\mathbb{Z})^{P}(\mathbb{Z})$,
   D is an intervals in $\mathbb{Z}$ if $D=\{a\}$ is a singleton or $|D|=2^K$ with $K\in \mathbb{N}^*$ and 
   there exist two sets $F_{\text{old}}(D),F_{\text{new}}(D)$ satisfying 
   $$|F_{\text{old}}(A)|=|F_{\text{new}}(D)|=2^{K-1},\ee D=F_{\text{old}}(D)\cup F_{\text{new}}(D)$$
   and $(F_{\text{old}}(D),F_{\text{old}},F_{\text{new}}),\ee (F_{\text{new}}(D),F_{\text{old}},F_{\text{new}})$  are Binary Russian Dolls (the definition is recursive). $F_{\text{old}},F_{\text{new}}$ are function taking the set of a Binary Russian Doll and returning its old or new subset Binary Russian Doll, these structural attributes are the specificties of a Binary Russian Doll compared to a simple Binary set. 
  \end{definition}
  The BRD structure is useful to define probabilities on set $D\subset \mathcal{P}(\Zset)$ such that $\log_2 |D|\in \Nset$, as we can see with the following definition.
  \begin{definition}
      Given a Binary Russian Doll $\text{Doll}=(D,F_{\text{old}},F_{\text{new}})$ and $R_1,R_2$ two functions $ \mathcal{P}(\mathbb{Z})^2 \to [0,1]$, the finite measure of probability $G_{(D,F_{\text{old}},F_{\text{new}}),R_1,R_2}$ 
      is defined on $D$ by $G_{(D,F_{\text{old}},F_{\text{new}}),R_1,R_2}(i)=\mathbbm{1}_a(i)$ when $D=\{a\}$ is a singleton and
      $$G_{(D,F_{\text{old}},F_{\text{new}}),R_1,R_2}(i)=R_1(F_{\text{old}}(D),F_{\text{new}}(D)))G_{(F_{\text{new}}(D),F_{\text{old}},F_{\text{new}}),R_2,R_2}(i)$$
      $$+(1-R_1(F_{\text{old}}(D),F_{\text{new}}(D))))G_{(F_{\text{old}}(D),F_{\text{old}},F_{\text{new}}),R_1,R_2}(i)$$
      otherwise, this definition is recursive.
  \end{definition}
  This definition gives us a general recipe to construct probabilities if we have a recipe to construct a BRD.
  In the \Cref{alg:practical} a BRD structure is implicitly used to define $\rmq_h$, we will try to shed light on this BRD construction.
  \begin{remark}
      For a given Binary Russian Doll $(D,F_{\text{old}},F_{\text{new}})$, only the values $F_{\text{old}}(N),F_{\text{new}}(N)$ when $N\subset D$ and $\log_2(|N|)\in \mathbb{N}$ are important (out of this condition $F_{\text{old}},F_{\text{new}})$ are not used).
      For $D$ a Binary Russian Doll $F_{\text{new}}(D),F_{\text{old}}(D)$ are apriori not uniquely determined given $D$, indeed $F_{\text{old}}(D)$ can be $[|\min D, \min D+ (\max D-\min D +1)//2-1|]$ or $[|\min D+ (\max D-\min D +1)//2, \max D|] $ (two possible choices)
  \end{remark}
  %Now we should explicit the construction of $(\msj,F_{\text{old}},F_{\text{new}})$ that the Algorithm used, more specifically we should define precisely $F_{\text{old}},F_{\text{new}}$. 
  The BRD implicitly used in \Cref{alg:practical} is defined thank to elementary specific BRD where $F_{\text{new}},F_{\text{old}}$  are uniquely determined.
  \begin{definition}
  Let $v\in \{0,1\}$. D set $D\subset \mathcal{P}(\mathbb{Z})$ is a $v$-monotone Binary Russian Doll, if $D=\{a\}$ is a singleton or A is a Binary Russian Doll with $|D|>1$ such that $A=F_{\text{old}}(D)\cup F_{\text{new}}(D)$ with $\max F_{\text{old}}(D)+1=\min  F_{\text{new}}(D)$ when $v=1$ (the older at left) or  $\max F_{\text{new}}(D)+1=\min  F_{\text{old}}(D)$ when $v=0$ (the older at right) and $F_{\text{old}}(D),F_{\text{new}}(D)$ $v$-monotone Binary Russian Doll (the definition is recursive).  $F_{\text{new}},F_{\text{old}}$ are here uniquely determined by $v$.
  
  $D$ is uniquely determined by its size $|A|$ and its minimum, thus we can note $D(m,k,v)$ the unique $v$-monotone Binary Russian Doll of size $2^k$ and minimum $m$.
  
  \end{definition}
  Thank to this definition, we can construct construct a BRD from a sequence of Bernoulli $(V_k)$.
  \begin{definition}
      Given a sequence $(v_k)\in\{0,1\}^L$ with $L\in \Nset^*$ and an integer $k\in [0,L]$, 
      we define the BRD $ \text{Doll}((v_i)_{0\leq i<L},k)=(I_k,F_{\text{old}},F_{\text{new}}) $ 
      such that if $k>0$,
      $$(F_{\text{old}}(I_k),F_{\text{old}},F_{\text{new}})=\text{Doll}((v_i)_{0\leq i<L},k-1)$$
      $$(F_{\text{new}}(I_k), F_{\text{old}},F_{\text{new}})=D(F(v_{k-1},I_{k-1}),k-1,v_{k-1}) $$
       where $F(v, I)=(\max I +1) \mathbbm{1}_1(v)+(\min I -|I|) \mathbbm{1}_0(v) $ for $I\subset{P}(\Zset )$ and $v\in \{0,1\}$
      (this function returns a value such that $F_{\text{old}}(I)\cup F_{\text{new}}(I)$ is an interval but $F_{\text{new}}(I)\cap F_{\text{old}}(I)=\{\} $), if $k=0$ $I_0=\{0\}$.
  \end{definition}
  
  \begin{remark}
      Let $L\in \Nset^*$. The sets $I_k$ for $k\in [0,L]$ in the previous defintion corresponds to the set of Algorithm 1 [[\ref{alg:nuts-doubling}]] at step $k$ related to the sequence of Bernoulli $(V_i)_{0\leq i<k}$.
  \end{remark}
  \begin{proof}
      In the last definition,
       we have the following relation thank to the $v$-monotone BRD and the definition of $F$: $I_k=I_{k-1}\cup [\max I_k +1, \max I_k +2^{k-1}]$ when $v_{k-1}=1$ 
       and $I_k=I_{k-1}\cup [\min I_k -2^{k-1}, \min I_k -1]$ when $v_{k-1}=0$, which is literally adding $2^k$ elements on the left or on the right to $I_k$, 
      the case $k=0$ is trivial.
  \end{proof}
  Now, to define $\rmq_h$ with $G_{(\msj,F_{\text{old}},F_{\text{new}}),R_1,R_2 }$, we should choose the functions $R_1$ and $R_2$.
  In the Stan implementation they choose the function $R_2$ to sample with a multinomial as suggests \Cref{prop:trajectory-invariance}, they use the following Lemma:
  %With these general definition we can define a wide range of probability on a set $\msj$ with Binary Russian Doll structure, it offers a general recipe for defining $\rmq_h $. 
  %Given two functions $R_1,R_2$, if we construct from $\msj,(q_0,p_0)$ a Binary Russian Doll $\text{Doll}=(\msj,F_{\text{old}},F_{\text{new}})$, we can define 
  %$$q(j|\msj,q_0,p_0)= G_{(\msj,F_{\text{old}},F_{\text{new}}),R_1,R_2 }(j) $$
   \begin{lemma}
      \label{lemma:mutinomal_G}
      Given a BRD $(D,F_{\text{old}},F_{\text{new}})$ and $R : \mathcal{P}(\Zset)^2\to [0,1]$ 
      such that $R(A,B)=\frac{\tpi(B)}{\tpi(A)+\tpi(B)}$ when $A,B$ are finite else $R(A,B)=0$. We have
      $$G_{(D,F_{\text{old}},F_{\text{new}}),R,R }(j)=\frac{\mathbbm{1}_D(j)\tpi(\Phiverlet[h][j](q_0,p_0))}{\sum_{i\in \msj}\tpi(\Phiverlet[h][i](q_0,p_0))}  $$
   \end{lemma}
   \begin{proof}
      We proceed by recurence using the relation
      $$G_{(D,F_{\text{old}},F_{\text{new}}),R,R}(j)=R(F_{\text{old}}(D),F_{\text{new}}(D))G_{(F_{\text{new}}(D),F_{\text{old}},F_{\text{new}}),R,R}(i)$$
  $$+(1-R(F_{\text{old}}(D),F_{\text{new}}(D)))G_{(F_{\text{old}}(D),F_{\text{old}},F_{\text{new}}),R,R}(i)$$
  Where the property indexed by $k\in \Nset$ is H(k):[the property of the lemma is true for BRD $(D,F_{\text{old}},F_{\text{new}})$ such that $|D|\leq 2^k $].
  k=0 is proven since by definition $G_{(D,F_{\text{old}},F_{\text{new}}),R,R }(j)=\mathbbm{1}_D(j)$ when $D$ is a singleton.
  Let $k\in \Nset$ such that $H(k)$ and let $(D,F_{\text{old}},F_{\text{new}})$ be a BRD with $|D|=2^{k+1}$.
  We have $|F_{\text{old}}(D)|=2^k$ and $|F_{\text{new}}(D)|=2^k$. We can apply $H(k)$ on $(F_{\text{old}}(D),F_{\text{old}},F_{\text{new}})$ and $(F_{\text{new}}(D),F_{\text{old}},F_{\text{new}})$:
  $$G_{(D,F_{\text{old}},F_{\text{new}}),R,R}(i)=R(F_{\text{old}}(D),F_{\text{new}}(D)) \frac{\mathbbm{1}_{F_{\text{new}}(D)}(j)\tpi(\Phiverlet[h][j](q_0,p_0))}{\sum_{i\in F_{\text{new}}(D)}\tpi(\Phiverlet[h][i](q_0,p_0)) } $$
  $$+(1-R(F_{\text{old}}(D),F_{\text{new}}(D)))\frac{\mathbbm{1}_{F_{\text{old}}(D)}(j) \tpi(\Phiverlet[h][j](q_0,p_0))}{\sum_{i\in F_{\text{old}}(D)}\tpi(\Phiverlet[h][i](q_0,p_0)) } $$
  $$ =\frac{(\mathbbm{1}_{F_{\text{new}}(D)}(j)+\mathbbm{1}_{F_{\text{old}}(D)}(j))\tpi(\Phiverlet[h][j](q_0,p_0))}{\sum_{i\in F_{\text{old}}(D) }\tpi(\Phiverlet[h][i](q_0,p_0))+\sum_{i\in F_{\text{new}}(D) }\tpi(\Phiverlet[h][i](q_0,p_0)) }  $$
  which proves the result since $F_{\text{new}}(D)\cup F_{\text{old}}(D)=D $.
  $\forall k\in \Nset :H(k)$.
  
   \end{proof}
   $R_2$ appears in the function BuildTree \ref{alg:practical} for this purpose.
   \begin{remark}
      \label{remark:multinomial_buildtree}
      Let $k\in [0,\Kmax]$, in \Cref{alg:practical}, we have $\theta_k'=\Phiverlet[h][j'](q_0,p_0)$ where $j'$ is sampled in $I^\text{new}_k=[\max I_k +1, \max I_k +2^{k-1}]$ when $V_k=1$ and
      $I^\text{new}_k=[\min I_k -2^{k-1}, \min I_k -1]$ when $V_k=0$ according to the multinomial $\bar{\pi}(.|I^\text{new}_k,q_0,p_0)$
   \end{remark}
   \begin{proof}
      Let $k\in [0,\Kmax]$, we can observe that the scheme of sampling for $j'$ in Buildtree$(.,k)$ follows the structure of $G_{D(F(V_{k},I_{k}),k,V_{k}),R,R }$ where $R$ is defined in the last \Cref{lemma:mutinomal_G}.
   \end{proof}
  
  %faire une preuve correcte en utilisant l'algo récursif? Rajouter schéma

  The following proposition legitimates the introduction of the Algorithm 3 [[\Cref{alg:nuts-samplingj}]]
  to sample the index.
  %remplacer par la relation de récurrence généré par l'algo update
  % à refaire proprement
  \begin{proposition}
  Given a sequence of bernouilli $V=(V_k)\in \{0,1\}^{\Kmax} $ such that $S=S((V_k),q_0,p_0)$ be the stopping time of the No U-turn sampler. We denote by $K_f=S-1\wedge \Kmax$ and $\msj =B_{K_f}(V|_{K_f})$
   %$\text{Doll}((v_i)_{0\leq i<K_f},K_f)=(\msj,F_{\text{old}},F_{\text{new}})$ the Binary Russian Doll that the algorithm returns when beginning from $q_0,p_0$ and
   and we define $R_1(I_1,I_2)=1\wedge \frac{\tpi(I_2)}{\tpi(I_1)}$ and  $R_2(I,\msj)= \frac{\tpi(I_2)}{\tpi(I_1)+\tpi(I_2)} $.
  In the Stan's implementation of the no U-turn HMC the index selection kernel $\rmq_h$ are:
  $$q(j|\msj,q_0,p_0)= G_{\text{Doll}((v_i)_{0\leq i<K_f},K_f),R_1,R_2}(j)$$
  which implies the following recurcive formula:
  $$q(j|\msj,q_0,p_0)=1\wedge \frac{\tpi(F_{\text{new}}(\msj))}{\tpi(F_{\text{old}}(\msj))} \frac{\mathbbm{1}_\msj(j)\tpi(\Phiverlet[h][j](q_0,p_0))}{\sum_{i\in F_{\text{new}}(\msj)}\tpi(\Phiverlet[h][i](q_0,p_0))} $$
  $$+(1-1\wedge \frac{\tpi(F_{\text{new}}(\msj))}{\tpi(F_{\text{old}}(\msj))}) G_{(F_{\text{old}}(\msj),F_{\text{old}},F_{\text{new}}),R_1,R_2}(j)$$
  \end{proposition}
  \begin{proof}
      Let $k\in [1,\Kmax]$, in \Cref{alg:practical}, we observe that 
      $\Sigma(\pi)_k$ is updated (Line 12) at the end of step $k$ such that $\Sigma(\pi)_k=\tilde{\pi}(I_k) $ since $\Sigma(\pi)_k' $ (returned by BuildTree) equals $\tilde{\pi}([\max I_k +1, \max I_k +2^{k-1}])$ when $V_k=1$ and $\tilde{\pi}([\min I_k -2^{k-1} , \min I_k -1]) $ when $V_k=0$.
      We have $\theta=\Phiverlet[h][j]$ where $j$ is sampled according to $G_{\text{Doll}((v_i)_{0\leq i<K_f},K_f),R_1,R_2}$ when the algorithm stops at step $K_f$, because of the multinomial sampling done in BuildTree according to \Cref{remark:mutinomial_buildtree} and the acceptation of the multinomial
      proposition with probability $1\wedge \frac{\Sigma(\pi)_k'}{\Sigma(\pi)_k}$ at Line 10 in \Cref{alg:practical}.
  %mettre des k de partout pour les variables
  \end{proof}

  \begin{figure}[!h]
      \begin{center}
      \includegraphics[width=100mm]{images/old_new_0.png}
      \end{center}
      \caption{Illustration of the construction of the structured sets when starting from $z_0$ where $z_i=\Phiverlet[h][i](z_0)$}
      \label{scheme_old_new_0}
  \end{figure}
  
  \begin{figure}[!h]
      \begin{center}
      \includegraphics[width=100mm]{images/old_new.png}
      \end{center}
      \caption{Scheme of the construction of the structured sets when starting from $z_3$ where $z_i=\Phiverlet[h][i](z_0)$}
      \label{scheme_old_new_3}
  \end{figure}
  
  \begin{figure}[!h]
      \begin{center}
      \includegraphics[width=100mm]{images/scheme_prob_bad.png}
      \end{center}
      \caption{Illustration of the construction of the probability $\rmq_h$}
      \label{scheme_prob_bad}
  \end{figure}
